# Supplementary material for: Landau levels in strained two-dimensional photonic crystals
Source: arXiv:2003.06690 ancillary file (2020-03-14)
Supplement: Supplementary file 1 [file Supplemental_Materials.pdf]

# LANDAU LEVELS IN STRAINED TWO-DIMENSIONAL PHOTONIC CRYSTALS: SUPPLEMENTAL MATERIALS

J. GUGLIELMON, M. RECHTSMAN AND M. I. WEINSTEIN

## 1. Overview

Here we give a detailed derivation of the results presented in the main text. Starting with a general class of continuum partial differential equations, which includes the single particle Schrödinger equation and the Maxwell equations for 2D photonic crystals (we treat both TE and TM polarization), we apply a multiple scale perturbation analysis to non-uniformly deformed honeycomb structures to derive the effective equations governing wave packets that are constructed from states with energies near $E_D$ (the energy of the Dirac point in the undeformed structure). The resulting effective Hamiltonian is a Dirac Hamiltonian with an *effective magnetic potential* and an *effective electric potential*, both generated by the prescribed deformation. We derive expressions for all parameters of the effective theory in terms of the bulk modes of the unstrained structure. The theory contains no free parameters. Our arguments work for arbitrary finite contrast and no tight-binding regime is required. The analysis can be adapted to other wave equations, *e.g.* acoustics, elasticity. We also provide details relating to the particular deformations discussed in the main text, which are designed to generate a flat Landau level spectrum.

## 2. Bulk honeycomb structure

We consider wave equations which arise in quantum and classical physics,

the *Schrödinger equation:*

$$i\partial_t\Psi \ = \ H\Psi \ = \ (-\Delta + V(\mathbf{x}))\,\Psi. \tag{2.1}$$

and the *classical wave equation*:

$$c^{-2}\ \rho(\mathbf{x})\ \partial_t^2\Psi\ - \nabla_{\mathbf{x}}\cdot\xi(\mathbf{x})\nabla_{\mathbf{x}}\Psi \ = \ 0. \tag{2.2}$$

In the above equations, $V(\mathbf{x})$ is real-valued, $\rho(\mathbf{x})$ is real-valued and strictly positive, and $\xi(\mathbf{x})$ is a symmetric $2\times 2$ matrix whose eigenvalues are bounded away from zero, uniformly in $\mathbf{x}$. For simplicity, $\xi(\mathbf{x})$ , $\rho(\mathbf{x})$ and $V(\mathbf{x})$ are taken to be smooth in $\mathbf{x}$.

Time-harmonic solutions, $\Psi(\mathbf{x},t) = e^{-i\omega t}\psi(\mathbf{x})$, are determined by the solutions of the Helmholtz / Schrödinger spectral problem:

$$(\ -\nabla_{\mathbf{x}}\cdot\xi(\mathbf{x})\nabla_{\mathbf{x}}\ +\ V(\mathbf{x})\ )\,\psi \ = \ E\ \rho(\mathbf{x})\psi \tag{2.3}$$

where we have combined the Schrödinger and classical cases to facilitate a unified treatment of Eqs. (2.1) and (2.2). In particular, the time-independent equation (2.3) incorporates several cases of interest:

(1) Schrödinger: $\xi(\mathbf{x}) = I_{2\times 2}$, $\rho(\mathbf{x}) \equiv 1$, $V(\mathbf{x}) =$ potential.
(2) Maxwell TM: $\xi(\mathbf{x}) = I_{2\times 2}$, $\rho(\mathbf{x}) = \varepsilon(\mathbf{x})$, $V(\mathbf{x}) = 0$, $E = (\omega/c)^2$.

(3) Maxwell TE: $\xi(\mathbf{x}) = [\varepsilon(\mathbf{x})]^{-1}$, $\rho(\mathbf{x}) = 1$, $V(\mathbf{x}) = 0$, $E = (\omega/c)^2$.
We may write (2.3) as

$$\mathcal{L}_{\xi,\rho}\,\psi \;=\; E\,\psi, \qquad \text{where} \qquad \mathcal{L}_{\xi,\rho} \;=\; \frac{1}{\rho(\mathbf{x})}\Big( -\nabla_{\mathbf{x}}\cdot\xi(\mathbf{x})\nabla_{\mathbf{x}} \;+\; V(\mathbf{x}) \Big). \tag{2.4}$$

Consider the case where $\xi(\mathbf{x}), \rho(\mathbf{x})$ and $V(\mathbf{x})$ are periodic with respect to a lattice, $\Lambda = \mathbb{Z}\mathbf{v}_1 \oplus \mathbb{Z}\mathbf{v}_2 \subset \mathbb{R}^2_{\mathbf{x}}$, where $\mathbf{v}_i$ are the lattice vectors. We denote a choice of unit cell by $\Omega$, the dual lattice by $\Lambda^*$, and a dual unit cell in $\mathbb{R}^2_{\mathbf{k}}$ by $\mathcal{B}$ (Brillouin zone). $\mathcal{L}_{\xi,\rho}$ is self-adjoint with respect to the inner product [1]

$$\langle f, g\rangle_\rho \;=\; \int_\Omega \overline{f(\mathbf{x})}g(\mathbf{x})\;\rho(\mathbf{x})\;d\mathbf{x}.$$

and has a (Bloch) band spectrum. We denote its bands by:

$$E_1(\mathbf{k}) \le E_2(\mathbf{k}) \le \cdots \le E_b(\mathbf{k}) \le \dots, \qquad \mathbf{k} = (k_1, k_2) \in \mathcal{B}.$$

*Remark* 2.1. For Maxwell's equations ($V = 0$), $\mathcal{L}_{\xi,\rho}$ is a non-negative self-adjoint operator and hence $E_b(\mathbf{k}) \ge 0$ for all $b \ge 1$. Since $(\omega/c)^2 = E$, there are two families of bands given by: $\omega_{b,\pm}(\mathbf{k}) \;=\; \pm c\sqrt{E_b(\mathbf{k})}$. For simplicity, we focus on the positive branch.

2.1. **Bulk honeycomb media.** Assume now that $\Lambda$ denotes the equilateral triangular lattice in $\mathbb{R}^2$. For each $\mathbf{v} \in \Lambda$ let $T_{\mathbf{v}}[f](\mathbf{x}) = f(\mathbf{x}+\mathbf{v})$. We say that $\mathcal{L}_{\xi,\rho}$, defined in (2.4), models a *bulk honeycomb medium* if:

$$[T_{\mathbf{v}}, \mathcal{L}_{\xi,\rho}] = 0, \quad \text{for all } \mathbf{v} \in \Lambda$$
$$[\mathcal{C}, \mathcal{L}_{\xi,\rho}] = 0, \quad [\mathcal{P}, \mathcal{L}_{\xi,\rho}] = 0, \quad [\mathcal{R}, \mathcal{L}_{\xi,\rho}] = 0.$$

Here, $\mathcal{C}[f](\mathbf{x}) = \overline{f(\mathbf{x})}$, $\mathcal{P}[f](\mathbf{x}) = f(-\mathbf{x})$ and $\mathcal{R}[f](\mathbf{x}) = f(R^*\mathbf{x})$, where $R$ is a $2\times 2$ matrix of rotation by $2\pi/3$. That is, the coefficients of $\mathcal{L}_{\xi,\rho}$ are $\Lambda-$ periodic, real-valued and, with respect to some origin of coordinates (taken to be $\mathbf{x}_0 = 0$) inversion-symmetric and $2\pi/3-$ rotationally invariant. With regard to $\xi(\mathbf{x})$, we focus on the isotropic case:

$$\xi = \xi(\mathbf{x})\; I_{2\times 2}, \quad \text{where } \mathcal{R}[\xi](\mathbf{x}) = \xi(R^*\mathbf{x}) = \xi(\mathbf{x}). \tag{2.5}$$

Note that the above definition of bulk honeycomb media includes structures that are more general than just an ordinary honeycomb lattice of discrete sites. Any structure that satisfies the symmetries (e.g. a triangular lattice of pillars) is included in the definition.

2.2. **Dirac points.** A Dirac point is an energy / quasi-momentum pair, $(E_D, \mathbf{K}_\star)$, at which there is a conical intersection of consecutive dispersion surfaces $E_-(\mathbf{k}) \le E_+(\mathbf{k})$:

$$E_\pm(\mathbf{k}) - E_D \;= \pm \mathrm{v_D}\;\; |\mathbf{k}-\mathbf{K}_\star|\;\;(\,1\;+\;O\left(|\mathbf{k}-\mathbf{K}_\star|\right)\,)\,, \quad \text{as}\;\; |\mathbf{k}-\mathbf{K}_\star| \to 0. \quad (\mathrm{v} > 0).$$

In Fig. 1, we show the honeycomb photonic crystal discussed in the main text along with its band structure, which exhibits a Dirac point between the first and second TE bands.

**Theorem 2.2.** *Generic bulk honeycomb operators of the type $\mathcal{L}_{\xi,\rho}$ (see* (2.4)*) have Dirac points at the vertices of the Brillouin zone.*

See [3,4] for the Schrödinger case and [6] for the Maxwell case. In the following discussion, we shall follow the mathematical formulations of these references.

[1]Note that, in the main text, we use Dirac notation for inner products $\langle f|g\rangle = \langle f, g\rangle$. Throughout this Supplemental Material, we will use the latter notation.

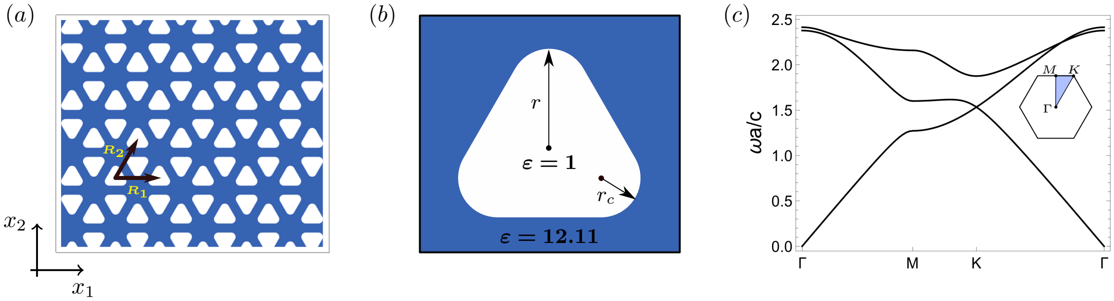


FIGURE 1. Illustration of the unstrained honeycomb photonic crystal discussed in the main text. (a) A portion of the periodic structure consisting of triangular air holes embedded in silicon. Shown also are the lattice vectors $\mathbf{R}_1 = a[1,0]$ and $\mathbf{R}_2 = a[1/2, \sqrt{3}/2]$. (b) Enlarged view of a single triangular air hole highlighting the values of the dielectric as well as the parameters $r$ and $r_c$ discussed in the main text. (c) TE bands of the structure, showing the Dirac point occurring between the first and second bands. Inset shows the Brillouin zone.

2.3. **Characterization of Dirac points.** Let

$$L^2_{\mathbf{k}} = \left\{ f : f(\mathbf{x}+\mathbf{v}) = e^{i\mathbf{k}\cdot\mathbf{v}} f(\mathbf{x}), \int_\Omega |f(\mathbf{x})|^2 \, \rho(\mathbf{x}) \, d\mathbf{x} < \infty \right\}, \quad \Omega = \text{unit cell.} \tag{2.6}$$

The inner product on $L^2_{\mathbf{k}}$ is given by:

$$\langle f, g \rangle_\rho = \int_\Omega \overline{f(\mathbf{x})} g(\mathbf{x}) \, \rho(\mathbf{x}) \, d\mathbf{x}, \quad \Omega = \text{unit cell.} \tag{2.7}$$

It will also be useful to introduce the standard $L^2$ inner product on a unit cell, which we denote by:

$$\langle f, g \rangle = \int_\Omega \overline{f(\mathbf{x})} g(\mathbf{x}) \, d\mathbf{x}, \quad \Omega = \text{unit cell.} \tag{2.8}$$

Introduce the subspaces $L^2_{\mathbf{K}_\star,\sigma}$ for $\sigma = 1, \tau, \bar{\tau}$ given by

$$L^2_{\mathbf{K}_\star,\sigma} = \left\{ f : f \in L^2_{\mathbf{K}_\star}, \ \mathcal{R}[f] = \sigma f \right\}. \tag{2.9}$$

Then, we have an orthogonal decomposition of $L^2_{\mathbf{K}_\star}$:

$$L^2_{\mathbf{K}_\star} = L^2_{\mathbf{K}_\star,1} \oplus L^2_{\mathbf{K}_\star,\tau} \oplus L^2_{\mathbf{K}_\star,\bar{\tau}}$$

For any vertex $\mathbf{K}_\star$ of the Brillouin zone, $[\mathcal{R}, L_{\xi,\rho}]$ acts in $L^2_{\mathbf{K}_\star}$ and vanishes. Hence, we may study the bulk honeycomb operator, $L_B$, on each summand subspace. We have the following characterization of Dirac points.

**Proposition 2.3.** *Let $\mathcal{L}_{\xi,\rho}$ be as defined in* (2.4). *Let $\mathbf{K}_\star = \mathbf{K}$ or $\mathbf{K}'$, the two independent high-symmetry vertex quasi-momenta of $\mathcal{B}$. The energy / quasi-momentum pair $(E_D, \mathbf{K}_\star)$ is a Dirac point (conical point) of $\mathcal{L}_{\xi,\rho}$ if:*

- *$E_D$ is a simple $L^2_{\mathbf{K}_\star,\tau}$ eigenvalue of $\mathcal{L}_{\xi,\rho}$ with corresponding eigenstate $\Phi_1(\mathbf{x})$ satisfying: $\mathcal{L}_{\xi,\rho}\Phi_1 = E_D\Phi_1$, $\mathcal{R}[\Phi_1] = \tau \, \Phi_1$.*

- *$E_D$ is a simple $L^2_{\mathbf{K}_\star,\overline{\tau}}$ eigenvalue of $\mathcal{L}_{\xi,\rho}$ with corresponding eigenstate $\Phi_2(\mathbf{x})$ satisfying: $\mathcal{L}_{\xi,\rho}\Phi_2 = E_D\Phi_2$, $\mathcal{R}[\Phi_2] = \overline{\tau}\ \Phi_2$.*
- *$\Phi_1$ and $\Phi_2$ are related by:*

$$\Phi_2(\mathbf{x}) = (\mathcal{PC})\,[\Phi_1](\mathbf{x}) = \overline{\Phi_1(-\mathbf{x})} \qquad \text{and} \quad \langle \Phi_j, \Phi_l \rangle_\rho = \delta_{jl}. \tag{2.10}$$

- *$E_D$ is not a $L^2_{\mathbf{K}_\star,1}$ eigenvalue of $\mathcal{L}_{\xi,\rho}$.*

*Furthermore, when the above conditions hold, we have the following: Let $\Phi_j^{\mathbf{K}_\star}$, $j = 1,2$ denote the pair of eigensolutions for $\mathbf{K}_\star = \mathbf{K}$ or $\mathbf{K}'$. Then, for some constant, $\mathrm{v_D}$, we have*

$$\left\langle \Phi_1^{\mathbf{K}}, \mathcal{A}\Phi_2^{\mathbf{K}} \right\rangle \ = \ \mathrm{v_D} \begin{pmatrix} 1 \\ i \end{pmatrix} \ , \tag{2.11}$$

*where $\mathcal{A}$ is given by:*

$$\mathcal{A} \ = \ \frac{1}{i}\nabla_{\mathbf{y}}\left(\xi(\mathbf{y})\cdot\right) \ + \ \xi(\mathbf{y})\frac{1}{i}\nabla_{\mathbf{y}} \ . \tag{2.12}$$

See Theorem 4.1 of [3], Theorem 2 of [6] and Section 3.1 of [1].

*Remark* 2.4. Note that if $\Phi_1$ and $\Phi_2$ are a choice of Bloch modes for the Dirac point $(E_D, \mathbf{K}_\star)$ satisfying all conditions of Proposition 2.3, then so are $e^{i\phi}\Phi_1$ and $e^{-i\phi}\Phi_2$ for any $\phi \in \mathbb{R}$. We shall take advantage of this degree of freedom in the proof of Proposition 2.5, where we choose a phase convention and coordinate system in which our effective equations take on a simplified form.

**Proposition 2.5.** *There is a coordinate system and a phase convention for the states $\Phi_1$ and $\Phi_2$ such that:*

$$\mathrm{v_D} = \langle \Phi_1, \mathcal{A}_1\Phi_2 \rangle \geq 0 \tag{2.13}$$

$$b_\star \ \equiv \ \langle \partial_{x_1}\Phi_1, \ \xi \ \partial_{x_1}\Phi_2 \rangle \ \geq \ 0. \tag{2.14}$$

The proof of Proposition 2.5 is given in Appendix B. It is dependent on Proposition 4.3 in Section 4, where the expression $b_\star$ arises in the derivation of the effective Hamiltonian.

N.B Henceforth, we shall assume throughout that $\mathrm{v_D} > 0$ and $b_\star > 0$.

We note that, for the structure studied numerically in the main text, the choice of coordinate system illustrated in Fig. 1(a) (paired with an appropriate choice of phase convention) was found from numerical simulations to produce a real-valued $v_D$ and $b_\star$. We also note that in [3, 6] it is shown that $\mathrm{v_D}$ is generically non-zero. We believe that the same techniques can be used to show that both $\mathrm{v_D}$ and $b_\star$ are generically non-zero.

## 3. The deformed bulk honeycomb medium

We start with a bulk honeycomb (unstrained) medium, whose modes are solutions to the eigenvalue problem:

$$(\ -\nabla_{\mathbf{x}}\cdot\xi(\mathbf{x})\nabla_{\mathbf{x}} \ + \ V(\mathbf{x})\ )\,\psi \ = \ E\rho(\mathbf{x})\psi \tag{3.1}$$

We subject the medium to a strain which is non-uniform on a length scale which is large compared with the lattice constant of the structure, denoted $a$:

$$\mathbf{x} \mapsto T(\mathbf{x}) \ \equiv \ \mathbf{x} \ + \ \mathbf{u}(\kappa\mathbf{x}), \quad \kappa a \ll 1,$$

where $\mathbf{u}(\mathbf{X}) = (u_1(\mathbf{X}), u_2(\mathbf{X}))$ and $\mathbf{X} = (X_1, X_2)$ [2]. The Jacobian of $T$ is given by $D_\mathbf{x}T(\mathbf{x}) = I_{2\times 2} + \kappa D_\mathbf{X}\mathbf{u}(\mathbf{X})\Big|_{\mathbf{X}=\kappa\mathbf{x}}$, where:

$$\left[D_\mathbf{X}\mathbf{u}(\mathbf{X})\right]_{jl} \equiv \left(\frac{\partial u_j(X_1,X_2)}{\partial X_l}\right)_{j,l=1,2} \equiv \left(u_{j,l}\right)_{j,l=1,2} \tag{3.2}$$

is the $2\times 2$ Jacobian matrix. If $\|D_\mathbf{X}\mathbf{u}(\mathbf{X})\|$ is bounded, then $T$ is invertible for $\kappa$ small.

We note that the deformation that we choose later on (corresponding to a constant pseudo-magnetic field) arises from a strain that grows linearly: $\left|\left(D_\mathbf{X}\mathbf{u}(\mathbf{X})\right)_{jl}\right| \sim a|\mathbf{X}|$. In this case, our asymptotic analysis is, strictly speaking, no longer valid at large distances: $|\mathbf{X}| \gg (\kappa a)^{-1}$. However, near the center of the band at $k_y a' = 0$ (see Fig. 2(b) of the main text), the Landau level wavefunctions are localized near $\mathbf{X} = \mathbf{0}$, and thus are supported only where the strain is weak. We therefore expect the $\mathcal{O}(\kappa)$ asymptotic analysis to be accurate up to $\mathcal{O}(\kappa^2)$ corrections in this regime (i.e. for $\mathbf{X} \approx \mathbf{0}$ and $k_y a'$ close to 0) [3].

The deformed medium is defined by primed material relations:

$$\xi'(T(\mathbf{x})) = \xi(\mathbf{x}), \quad V'(T(\mathbf{x})) = V(\mathbf{x}), \quad \rho'(T(\mathbf{x})) = \rho(\mathbf{x}),$$

Assuming that $T$ is invertible we have

$$\xi'(\mathbf{x}) = \xi(T^{-1}(\mathbf{x})), \quad V'(\mathbf{x}) = V(T^{-1}(\mathbf{x})), \quad \rho'(\mathbf{x}) = \rho(T^{-1}(\mathbf{x})),$$

The spectral problem governing modes of the deformed medium is then:

$$\left( -\nabla_\mathbf{x} \cdot \xi'(\mathbf{x})\nabla_\mathbf{x} + V'(\mathbf{x}) \right)\psi = E\rho'(\mathbf{x})\psi. \tag{3.3}$$

Introducing the change of variables and definitions

$$\begin{aligned} \mathbf{y} &= T^{-1}(\mathbf{x}) \\ J(\mathbf{y}) &\equiv D_\mathbf{x}T^{-1}(\mathbf{x})\Big|_{\mathbf{x}=T(\mathbf{y})} = \left[\partial_\mathbf{y}T(\mathbf{y})\right]^{-1}, \qquad |J(\mathbf{y})| \equiv \det J(\mathbf{y}) \end{aligned}$$

we obtain an equivalent equation to (3.3) in terms of the undeformed material functions:

$$-\left[|J(\mathbf{y})|\nabla_\mathbf{y} \cdot \frac{J(\mathbf{y})\xi(\mathbf{y})J^\top(\mathbf{y})}{|J(\mathbf{y})|}\nabla_\mathbf{y}\right]\psi + V(\mathbf{y})\,\psi = E\rho(\mathbf{y})\psi. \tag{3.4}$$

For the undeformed problem, $\kappa = 0$, (3.4) reduces to (3.1).

We next expand the equation (3.4) in the small parameter $\kappa$ and drop terms of order $\kappa^2$ and higher order. For simplicity we consider the isotropic case:

$$\xi = \xi(\mathbf{x})I_{2\times 2}. \tag{3.5}$$

[2]NB: Here we take the deformation to be of the form $\mathbf{u}(\kappa\mathbf{x})$ instead of $\mathbf{u}(x)$ (compare with the main text). In doing so we are explicitly introducing the small parameter measuring the size of the deformation in order to facilitate our systematic perturbation theory.

[3]We conjecture that a physical regularization of the structure (one in which the structure is undeformed for $|x_1|$ sufficiently large), will yield high density of states near the degenerate Landau levels of the present asymptotic theory. A mathematically rigorous treatment is work in progress.

Since $T(\mathbf{y}) = \mathbf{y} + \mathbf{u}(\kappa\mathbf{y})$, we have $D_{\mathbf{y}}T(\mathbf{y}) = I_{2\times 2} + \kappa D_{\mathbf{Y}}\mathbf{u}(\mathbf{Y})\Big|_{\mathbf{Y}=\kappa\mathbf{y}}$. Therefore,

$$\begin{aligned} J(\mathbf{y}) &= I_{2\times 2} - \kappa D_{\mathbf{Y}}\mathbf{u}(\mathbf{Y})\Big|_{\mathbf{Y}=\kappa\mathbf{y}} + \mathcal{O}(\kappa^2) \\ &= \begin{pmatrix} 1-\kappa u_{1,1} & -\kappa u_{1,2} \\ -\kappa u_{2,1} & 1-\kappa u_{2,2} \end{pmatrix}\Big|_{\mathbf{Y}=\kappa\mathbf{y}} + \mathcal{O}(\kappa^2) \end{aligned} \tag{3.6}$$

and

$$|J(\mathbf{y})| = 1 - \kappa\, \nabla_{\mathbf{Y}} \cdot \mathbf{u}(\mathbf{Y})\Big|_{\mathbf{Y}=\kappa\mathbf{y}} + \mathcal{O}(\kappa^2) \tag{3.7}$$

We next expand (3.4) using

$$\begin{aligned} |J|\nabla_{\mathbf{y}} \cdot \frac{J\xi J^\top}{|J|}\, \nabla_{\mathbf{y}} &= \nabla_{\mathbf{y}} \cdot J\xi J^\top\, \nabla_{\mathbf{y}} + |J| \left(\nabla_{\mathbf{y}}|J|^{-1}\right) \cdot \left(J\xi J^\top\, \nabla_{\mathbf{y}}\right) \\ &= \nabla_{\mathbf{y}} \cdot J\xi J^\top\, \nabla_{\mathbf{y}} + \mathcal{O}(\kappa^2) \end{aligned} \tag{3.8}$$

and

$$\begin{aligned} J\xi J^\top &= \left( I_{2\times 2} - \kappa D_{\mathbf{Y}} u \right)\, \xi\, \left( I_{2\times 2} - \kappa (D_{\mathbf{Y}} u)^\top \right) + \mathcal{O}(\kappa^2) \\ &= \xi - 2\,\kappa\,\xi\, U + \mathcal{O}(\kappa^2), \end{aligned} \tag{3.9}$$

where $U = (U_{ij})$, the strain matrix, with entries [4]

$$U_{ij}(\mathbf{Y}) = \frac{1}{2}\left( \frac{\partial u_i}{\partial Y_j} + \frac{\partial u_j}{\partial Y_i} \right) = \frac{1}{2}\left( D_{\mathbf{Y}}\mathbf{u}(\mathbf{Y}) + D_{\mathbf{Y}}\mathbf{u}(\mathbf{Y})^\top \right)_{ij} \tag{3.10}$$

Using (3.8), (3.9) and (3.10) in (3.4) yields:

$$\left( -\nabla_{\mathbf{y}} \cdot \xi(\mathbf{y})\, \nabla_{\mathbf{y}} + V(\mathbf{y}) \right)\psi + 2\,\kappa\, \nabla_{\mathbf{y}} \cdot \xi(\mathbf{y})\, U(\kappa\mathbf{y})\, \nabla_{\mathbf{y}}\, \psi = E\, \rho(\mathbf{y})\, \psi + \mathcal{O}(\kappa^2) \tag{3.11}$$

## 4. Effective equations via multiscale analysis

The form of the expanded Helmholtz / Schrödinger operator on the left hand side of (3.11) reflects the assumptions on our slowly deformed bulk structure; it depends on the two spatial scales: $\mathbf{y}$ (fast) and $\mathbf{Y} = \kappa\mathbf{y}$ (slow). To capture the $\kappa^{-1}$ length scale effect of the non-uniform deformation, we seek solutions which explicitly incorporate both of these scales:

$$\psi^\kappa(\mathbf{y}) = \Psi^\kappa\left(\mathbf{y}, \mathbf{Y}\right)\big|_{\mathbf{Y}=\kappa\mathbf{y}}\,, \tag{4.1}$$

where $\mathbf{y}$ and $\mathbf{Y}$ are to be treated as independent variables. Reflecting this, the solutions of (3.11) that we shall construct are approximate wavepackets consisting of bulk Bloch mode components with energies nearby the Dirac point $|E - E_D| \lesssim C\kappa$. The expansion procedure we present has been made mathematically rigorous in many settings; in the context of perturbed honeycomb structures, see for example, [1, 2, 6].

[4]Since, in these Supplemental Materials, we have explicitly introduced the small parameter $\kappa$, the $\kappa$ dependence of the strain matrix has been made explicit and is factored out of $U$ as defined above. The strain matrix defined in the main text thus differs from that defined here by a factor of $\kappa$ and is given by $\kappa U$.

First, we re-express (3.11) in terms of this extended set of variables: $(\mathbf{y}, \mathbf{Y})$. Thus we replace $\nabla_{\mathbf{y}}$ by $\nabla_{\mathbf{y}} + \kappa \nabla_{\mathbf{Y}}$ in (3.11). Keeping terms of order $\kappa^0$ and $\kappa^1$, we find that (3.11) becomes:

$$( \mathcal{L}_0 + \kappa \mathcal{L}_1 ) \Psi^\kappa(\mathbf{y}, \mathbf{Y}) = E \rho \Psi^\kappa(\mathbf{y}, \mathbf{Y}) + \mathcal{O}(\kappa^2)$$

where

$$\mathcal{L}_0 = -\nabla_{\mathbf{y}} \cdot \xi(\mathbf{y}) \nabla_{\mathbf{y}} + V(\mathbf{y}) \tag{4.2}$$

$$\mathcal{L}_1 = - ( \nabla_{\mathbf{y}} \cdot \xi(\mathbf{y}) \nabla_{\mathbf{Y}} + \nabla_{\mathbf{Y}} \cdot \xi(\mathbf{y}) \nabla_{\mathbf{y}} ) + 2 \nabla_{\mathbf{y}} \cdot \xi(\mathbf{y}) U(\mathbf{Y}) \nabla_{\mathbf{y}} \tag{4.3}$$

For each fixed $\mathbf{Y} \in \mathbb{R}^2$, the operators $\mathcal{L}_0$ and $\mathcal{L}_1$ are self-adjoint operators in $L^2_{\mathbf{K}}$.

We study the ($\mathcal{O}(\kappa)$ approximate) eigenvalue problem [5]

$$(\mathcal{L}_0 + \kappa \mathcal{L}_1) \Psi^\kappa = E \rho \Psi^\kappa, \tag{4.4}$$

$$\Psi^\kappa(\mathbf{y} + \mathbf{v}, \mathbf{Y}) = e^{i\mathbf{K}\cdot\mathbf{v}} \Psi^\kappa(\mathbf{y}, \mathbf{Y}), \tag{4.5}$$

with specified boundary conditions for $\Psi^\kappa(\mathbf{y}, \mathbf{Y})$ with respect to $\mathbf{Y}$. (4.6)

Seek a solution of (4.4)-(4.6) as an expansion:

$$\Psi^\kappa(\mathbf{y}, \mathbf{Y}) = \psi_0(\mathbf{y}, \mathbf{Y}) + \kappa \psi_1(\mathbf{y}, \mathbf{Y}) + \ldots \tag{4.7}$$

$$E^\kappa = E_0 + \kappa E_1 + \ldots, \tag{4.8}$$

where each $\psi_j(\mathbf{y}, \mathbf{Y})$ satisfies the boundary conditions (4.5)-(4.6). Substitution and equating like powers of $\kappa$ yields a hierarchy of equations. The first two of these are:

$$\mathcal{O}(\kappa^0): \quad ( -\nabla_{\mathbf{y}} \cdot \xi(\mathbf{y}) \nabla_{\mathbf{y}} + V(\mathbf{y}) - E_0 \rho(\mathbf{y}) ) \psi_0 = 0 \tag{4.9}$$

$$\mathcal{O}(\kappa^1): \quad ( -\nabla_{\mathbf{y}} \cdot \xi(\mathbf{y}) \nabla_{\mathbf{y}} + V(\mathbf{y}) - E_0 \rho(\mathbf{y}) ) \psi_1 = -\mathcal{L}_1 \psi_0 + E_1 \rho(\mathbf{y}) \psi_0 \tag{4.10}$$

The general solution, $\psi_0$, of (4.9) with boundary conditions (4.5)-(4.6) is:

$$\psi_0(\mathbf{y}, \mathbf{Y}) = \sum_{j=1}^{2} \alpha_j(\mathbf{Y}) \Phi_j(\mathbf{y}), \quad E_0 = E_D, \quad \text{where} \tag{4.11}$$

(a) $\Phi_j(\mathbf{y})$, $j = 1, 2$ span the two-dimensional $\mathbf{K}-$pseudoperiodic eigenspace of $\frac{1}{\rho(\mathbf{y})} \mathcal{L}_0$ with eigenvalue $E_0 = E_D$; see Theorem 2.2, and
(b) $\alpha_j(\mathbf{Y})$ are functions to be determined, which vary on the slow scale, $\mathbf{Y}$, and are chosen to satisfy the condition (4.6) in $\mathbf{Y}$.

Using (4.11) we have that (4.10) becomes the non-homogeneous equation:

$$\begin{aligned} &(-\nabla_{\mathbf{y}} \cdot \xi(\mathbf{y}) \nabla_{\mathbf{y}} + V(\mathbf{y}) - E_D \rho(\mathbf{y}) ) \psi_1 \\ &= \sum_{j=1}^{2} (-\mathcal{L}_1) ( \alpha_j(\mathbf{Y}) \Phi_j(\mathbf{y}) ) + E_1 \sum_{j=1}^{2} \alpha_j(\mathbf{Y}) \rho(\mathbf{y}) \Phi_j(\mathbf{y}), \end{aligned} \tag{4.12}$$

[5] At this stage we do not specify boundary conditions with respect to $\mathbf{Y} = (Y_1, Y_2)$. These are specified below and depend on our choice of deformation. Specifically, for deformations giving rise to a Landau-gauge vector potential with constant effective magnetic field we shall choose: $\psi$ to be pseudo-periodic with respect to $Y_2$ and decaying as $|Y_1| \to \infty$. See Section 5.

where $\psi_1$ satisfies the boundary conditions (4.5)-(4.6). Next, introduce the self-adjoint first order vector-operator

$$\mathcal{A} = \frac{1}{i}\nabla_{\mathbf{y}}\left(\xi(\mathbf{y})\cdot\right) + \xi(\mathbf{y})\frac{1}{i}\nabla_{\mathbf{y}}, \text{ or}$$
$$\mathcal{A} = (\mathcal{A}_1,\mathcal{A}_2), \text{ where } \mathcal{A}_l \equiv \frac{1}{i}\partial_{y_l}\left(\xi(\mathbf{y})\cdot\right) + \xi(\mathbf{y})\frac{1}{i}\partial_{y_l} \tag{4.13}$$

Then, the equation for $\psi_1$ may be rewritten as:

$$\begin{aligned}&\left(-\nabla_{\mathbf{y}}\cdot\xi(\mathbf{y})\ \nabla_{\mathbf{y}} + V(\mathbf{y}) - E_D\ \rho(\mathbf{y})\ \right)\psi_1\\ &= i\sum_{j=1}^{2}\mathcal{A}\Phi_j(\mathbf{y})\cdot\nabla_{\mathbf{Y}}\alpha_j(\mathbf{Y}) - 2\sum_{j=1}^{2}\nabla_{\mathbf{y}}\cdot\xi(\mathbf{y})\ U(\mathbf{Y})\ \nabla_{\mathbf{y}}\Phi_j(\mathbf{y})\ \alpha_j(\mathbf{Y})\\ &\quad + E_1\ \rho(\mathbf{y})\sum_{j=1}^{2}\Phi_j(\mathbf{y})\alpha_j(\mathbf{Y})\ .\end{aligned} \tag{4.14}$$

The non-homogeneous equation (4.14) is viewed as an equation for $\mathbf{y}\mapsto\psi_1(\mathbf{y},\mathbf{Y})$ satisfying the pseudoperiodic boundary condition (4.5). A necessary and sufficient condition for solvability is that the right hand side of (4.14) be $L^2$ orthogonal to the Dirac subspace of $\mathcal{L}_0 = -\nabla_{\mathbf{y}}\cdot\xi(\mathbf{y})\ \nabla_{\mathbf{y}} + V(\mathbf{y})$ at energy $E_D$, which is spanned by $\{\ \Phi_1,\Phi_2\ \}$. Thus we have,

**Proposition 4.1.** *Equation* (4.14) *for* $\psi_1(\mathbf{y},\mathbf{Y})$ *with boundary conditions* (4.5)-(4.6) *has a solution if and only if* $\alpha(\mathbf{Y}) = (\alpha_1(\mathbf{Y}),\alpha_2(\mathbf{Y}))^\top$ *satisfy the following eigenvalue problem for* $(\alpha(\mathbf{Y}),E_1)$ *subject to the boundary condition imposed in* (4.6) .

$$\begin{aligned}&-i\sum_{j=1}^{2}\langle\Phi_l,\mathcal{A}\Phi_j\rangle\cdot\nabla_{\mathbf{Y}}\alpha_j(\mathbf{Y}) + 2\sum_{j=1}^{2}\langle\Phi_l,\nabla_{\mathbf{y}}\cdot\xi\ U(\mathbf{Y})\ \nabla_{\mathbf{y}}\Phi_j\rangle\ \alpha_j(\mathbf{Y})\\ &= E_1\ \alpha_l(\mathbf{Y}), \quad \textit{for } l=1,2,\end{aligned} \tag{4.15}$$

*where we have used the normalization* $\langle\Phi_l,\rho\ \Phi_j\rangle = \delta_{lj}$*; see* (2.10).

We next write out explicitly the second term in (4.15):

$$\begin{aligned}2\ \langle\Phi_l,\nabla_{\mathbf{y}}\cdot\xi\ U(\mathbf{Y})\ \nabla_{\mathbf{y}}\Phi_j\rangle &= -2\ \langle\nabla_{\mathbf{y}}\Phi_l,\xi\ U(\mathbf{Y})\ \nabla_{\mathbf{y}}\Phi_j\rangle\\ &= -2\sum_m\left\langle\ \partial_{y_m}\Phi_l\ ,\ \xi\sum_n U_{mn}(\mathbf{Y})\ \partial_{y_n}\Phi_j\ \right\rangle\\ &= -2\sum_{m,n}U_{mn}(\mathbf{Y})\ \langle\ \partial_{y_m}\Phi_l\ ,\ \xi\ \partial_{y_n}\Phi_j\ \rangle\end{aligned} \tag{4.16}$$

4.1. **Simplification of the system** (4.15) **via application of symmetries.** Honeycomb symmetry enables simplification of the eigenvalue problem (4.15) for the pair $(\alpha,E_1)$. The coefficients in (4.15) are inner products of the form:

$$\langle\Phi_l,\zeta\cdot\mathcal{A}\Phi_j\rangle \quad \text{and} \quad A^{lj}_{\alpha\beta} = \left\langle\partial_{y_\alpha}\Phi_l,\xi\ \partial_{y_\beta}\Phi_j\right\rangle, \quad j,l,\alpha,\beta=1,2. \tag{4.17}$$

We next discuss their simplification using symmetry arguments. These results are then applied in Section 5 to obtain our effective equations.

The first type of inner product in (4.17) is evaluated using:

**Proposition 4.2.** *For $\zeta = (\zeta^{(1)}, \zeta^{(2)}) \in \mathbb{C}^2$, we have*

*(1)* $\langle \Phi_1, \zeta \cdot \mathcal{A}\Phi_1 \rangle = \overline{\langle \Phi_2, \zeta \cdot \mathcal{A}\Phi_2 \rangle} = 0.$

*(2)* $\langle \Phi_1, \zeta \cdot \mathcal{A}\Phi_2 \rangle = \overline{\langle \Phi_2, \zeta \cdot \mathcal{A}\Phi_1 \rangle} \ = \ \mathrm{v_D}\ (\zeta^{(1)} + i\zeta^{(2)}),$
*where* $\mathrm{v_D} = \frac{1}{2} \langle \Phi_1, \mathcal{A}\Phi_2 \rangle \cdot (1, -i)$*; see* (2.11).

Proposition 4.2 follows from Proposition 2.3; see also [1, 3, 6]. The second type of inner product in (4.17) is evaluated using the following proposition which is proved in Section A:

**Proposition 4.3.** *Let $A^{lj}$, with entries $A^{lj}_{\alpha\beta}$, be as defined in* (4.17)*:*

$$A^{lj}_{\alpha\beta} \ = \ \left\langle \partial_{y_\alpha} \Phi_l, \xi \ \partial_{y_\beta} \Phi_j \right\rangle, \quad j, l, \alpha, \beta = 1, 2.$$

*Then,*

*(1) for $l = j$:*

$$A^{jj} \ = \ a_\star \ I_{2\times2} \ + \ \tilde{a}^{jj} \begin{pmatrix} 0 & 1 \\ -1 & 0 \end{pmatrix} \ = \ a_\star \ \sigma_0 \ + \ i \ \tilde{a}^{jj} \ \sigma_2, \tag{4.18}$$

*where $\tilde{a}^{jj}$ are constants and $a_\star \geq 0$ and is given by*

$$a_\star \ = \ \langle \partial_{y_1} \Phi_1, \xi \ \partial_{y_1} \Phi_1 \rangle = \langle \partial_{y_2} \Phi_1, \xi \ \partial_{y_2} \Phi_1 \rangle \, , \quad \text{and} \tag{4.19}$$

$$a_\star \ = \ \langle \partial_{y_1} \Phi_2, \ \xi \ \partial_{y_1} \Phi_2 \rangle = \langle \partial_{y_2} \Phi_2, \xi \ \partial_{y_2} \Phi_2 \rangle \, . \tag{4.20}$$

*Moreover,*

$$a_\star \ = \ \frac{1}{2} \ E_D \ - \ \frac{1}{2} \ \int_\Omega V(\mathbf{y}) |\Phi_j(\mathbf{y})|^2 \, d\mathbf{y}, \ \ j = 1 \text{ or } 2. \tag{4.21}$$

*(2) for $l \neq j$:*

$$A^{12} \ = \ b_\star \begin{pmatrix} 1 & -i \\ -i & -1 \end{pmatrix} \ = \ b_\star \ ( \ \sigma_3 \ - \ i \ \sigma_1 \ ), \quad \textit{where} \quad b_\star = \langle \partial_{y_1} \Phi_1, \xi \ \partial_{y_1} \Phi_2 \rangle \tag{4.22}$$

$$A^{21} \ = \ \overline{A^{12}} \ = \ \overline{b_\star} \begin{pmatrix} 1 & i \\ i & -1 \end{pmatrix} \ = \ \overline{b_\star} \ ( \ \sigma_3 \ + \ i \ \sigma_1 \ ) \, . \tag{4.23}$$

Recall that by Proposition 2.5, a coordinate system and eigenstate phase convention can always be chosen for which: $\mathrm{v_D} \geq 0$ and $b_\star \geq 0$. The proof of Proposition 4.3 is given in Appendix A.

## 5. Pseudo-magnetic field and the effective equations

Using Proposition 4.2 and Proposition 4.3 we may greatly simplify the left hand side of (4.15). The detailed calculations are presented in Section 5.3; see, in particular, (5.13), (5.14), (5.17) and (5.18). This gives our main result:

**Theorem 5.1.** *(1) The eigenvalue problem* (4.15) *for $(\alpha, E_1)$ reduces to the eigenvalue problem, $\mathcal{H}\alpha \ = \ E_1\alpha$, where $\mathcal{H}$ is a Dirac Hamiltonian with effective magnetic and electric potentials:*

$$\mathcal{H} = \mathrm{v_D} \left[ ( \ -i\partial_{Y_1} \ - \ A_1 \ ) \, \sigma_1 \ - \ ( \ -i\partial_{Y_2} \ - \ A_2 \ ) \, \sigma_2 \right] \ + \ W_{\mathrm{eff}} \ \sigma_0. \tag{5.1}$$

*The effective electric potential,* $W_{\rm eff}$*, and effective magnetic potential,* $\mathbf{A}_{\rm eff} = (A_1, A_2)$*, are given by:*

$$W_{\rm eff}(\mathbf{Y}) = -2a_\star \ {\rm tr}\,(U(\mathbf{Y})\sigma_0) = \ -2a_\star\,(\partial_{Y_1}u_1 + \partial_{Y_2}u_2) \tag{5.2}$$

$$A_1(\mathbf{Y}) \ = \ +\frac{2b_\star}{{\rm v_D}}\ {\rm tr}\,(U(\mathbf{Y})\sigma_3) \ = \ +\frac{2b_\star}{{\rm v_D}}\ (\partial_{Y_1}u_1 - \partial_{Y_2}u_2) \tag{5.3}$$

$$A_2(\mathbf{Y}) \ = \ -\frac{2b_\star}{{\rm v_D}}\ {\rm tr}\,(U(\mathbf{Y})\sigma_1) = \ -\frac{2b_\star}{{\rm v_D}}\ (\partial_{Y_1}u_2 + \partial_{Y_2}u_1) \tag{5.4}$$

*where,* ${\rm v_D} > 0$, $a_\star \geq 0$ *and* $b_\star > 0$ *are constants given in terms of Bloch modes* $\Phi_1$, $\Phi_2$*:*

$$\begin{aligned}
{\rm v_D} \ &= \ \langle \Phi_1, \mathcal{A}_1 \Phi_2\rangle > 0. \\
a_\star \ &= \ \frac{1}{2}\ E_D \ - \ \frac{1}{2}\ \int_\Omega V(\mathbf{y})\ |\Phi_j(\mathbf{y})|^2\ d\mathbf{y} \ = \ \langle \partial_{y_1}\Phi_j,\ \xi\ \partial_{y_1}\Phi_j\rangle \geq 0,\ \ j = 1 \text{ or } 2 \\
b_\star \ &= \ \langle \partial_{y_1}\Phi_1,\ \xi\ \partial_{y_1}\Phi_2\rangle > 0.
\end{aligned}$$

(2) *Equivalently, the eigenvalue problem* (5.1) *may be expressed in terms of* $\alpha' \equiv \sigma_1\alpha = (\alpha_2, \alpha_1)^\top$ *and* $\mathcal{H}_{\rm eff} \equiv \sigma_1 \mathcal{H} \sigma_1^{-1}$ *as* $\mathcal{H}_{\rm eff}\alpha' = E_1\alpha'$*, where*

$$\mathcal{H}_{\rm eff} \ = \ {\rm v_D}\,(-i\nabla_{\mathbf{Y}} - \mathbf{A}_{\rm eff})\cdot\sigma \ + \ W_{\rm eff}\ \sigma_0 \ \ . \tag{5.5}$$

*Remark* 5.2. Note that for 2D electromagnetics ($V(\mathbf{x}) \equiv 0$) we have

$$a_\star = \frac{1}{2}\ E_D \ = \ \frac{1}{2}\ \left(\frac{\omega_D}{c}\right)^2.$$

*Remark* 5.3. Part (2) of Theorem 5.1 follows from part (1) and the observation that $\sigma_1\sigma_2\sigma_1^{-1} = -\sigma_2$, which implies that:

$$\begin{aligned}
\mathcal{H}_{\rm eff} &= \sigma_1 \left( {\rm v_D} \left[ (\ -i\partial_{Y_1} \ - \ A_1\ )\,\sigma_1 \ - \ (\ -i\partial_{Y_2} \ - \ A_2\ )\,\sigma_2 \right] \ + \ W_{\rm eff}\ \sigma_0 \ \right)\sigma_1^{-1} \\
&= \ {\rm v_D} \left[ \ (\ -i\partial_{Y_1} \ - \ A_1\ )\,\sigma_1 \ + \ (\ -i\partial_{Y_2} \ - \ A_2\ )\,\sigma_2 \ \right] \ + \ W_{\rm eff}\ \sigma_0 \\
&= \ {\rm v_D}\,(-i\nabla_{\mathbf{Y}} \ - \ \mathbf{A}_{\rm eff}) \ \cdot \sigma \ + \ W_{\rm eff}\ \sigma_0
\end{aligned}$$

This is equivalent to a relabeling of the pair of eigenmodes at the Dirac point: $\Phi_1 \mapsto \Phi_2$ and $\Phi_2 \mapsto \Phi_1$.

5.1. **Divergence-free deformations and Landau level spectrum.** Suppose that we constrain the deformation $\mathbf{u}(\mathbf{Y})$ by: ${\rm tr}\,(\sigma_0 U) \ = \ \nabla_{\mathbf{Y}}\cdot\mathbf{u} = 0$. Hence, $W_{\rm eff}(\mathbf{Y}) = 0$ and $\mathcal{H}_{\rm eff}$ takes the simpler form:

$$\mathcal{H}_{\rm eff} \ = \ {\rm v_D} \left[ (\ -i\partial_{Y_1} \ - \ A_1\ )\,\sigma_1 \ + \ (\ -i\partial_{Y_2} \ - \ A_2\ )\,\sigma_2 \ \right]. \tag{5.6}$$

Defining $\hat{\mathbf{p}} = (\hat{p}_1, \hat{p}_2) = (-i\partial_{Y_1}, -i\partial_{Y_2})$, we observe that $\mathcal{H}_{\rm eff}^2$ is a diagonal operator. Indeed,

$$\begin{aligned}
\mathcal{H}_{\rm eff}^2 \ &= \ {\rm v_D^2} \left[ \ (\hat{p}_1 - A_1)\sigma_1 \ + \ (\hat{p}_2 - A_2)\sigma_2 \ \right]^2 \\
&= \ {\rm v_D^2} \left[ \ (\hat{p}_1 - A_1)^2 \ + \ (\hat{p}_2 - A_2)^2 \ + \ (\hat{p}_1 - A_1)(\hat{p}_2 - A_2)\sigma_1\sigma_2 \ + \ (p_2 - A_2)(p_1 - A_1)\sigma_2\sigma_1 \ \right] \\
&= \ {\rm v_D^2} \left[ \ (\hat{\mathbf{p}} - \mathbf{A}_{\rm eff})^2 \ \sigma_0 + \ (\ \partial_{Y_2}A_1 - \partial_{Y_1}A_2\ ) \ \sigma_3 \ \right].
\end{aligned}$$

Hence,

$$\mathcal{H}_{\rm eff}^2 = {\rm v}_{\rm D}^2 \left[ (\hat{\mathbf{p}} - \mathbf{A}_{\rm eff})^2 \ \sigma_0 + \ V_{\rm eff}\ \sigma_3 \right], \text{ where} \tag{5.7}$$

$$V_{\rm eff} = -\left[\nabla_{\mathbf{Y}} \times \mathbf{A}_{\rm eff}\right] \cdot \hat{\mathbf{z}} = \partial_{Y_2} A_1 - \partial_{Y_1} A_2. \tag{5.8}$$

Now take $\mathbf{A}_{\rm eff}$ to be a Landau gauge vector potential for a constant magnetic field: $\mathbf{A}_{\rm eff} = -B_0\ (0, Y_1)$. Then, $\nabla \times \mathbf{A}_{\rm eff} = -B_0 \hat{\mathbf{z}}$. By (5.3)-(5.4), we must have:

$$A_1 = +\frac{2b_\star}{{\rm v}_{\rm D}} (u_{1,1} - u_{2,2}) = 0, \quad A_2 = -\frac{2b_\star}{{\rm v}_{\rm D}} (u_{1,2} + u_{2,1}) = -B_0\ Y_1 \ . \tag{5.9}$$

We solve equations (5.9) by taking:

$$\mathbf{u}(\mathbf{Y}) = (u_1(\mathbf{Y}), u_2(\mathbf{Y})) = \frac{{\rm v}_{\rm D}\ B_0}{4b_\star} \left(0, Y_1^2\right) .$$

From the above results, we have

$$\mathcal{H}_{\rm eff}^2 = {\rm v}_{\rm D}^2 \left[p_1^2 \sigma_0 + (p_2 + B_0 Y_1)^2 \sigma_0 + B_0 \sigma_3\right]. \tag{5.10}$$

This yields two decoupled copies of the Landau gauge Hamiltonian for a particle in a magnetic field, with the copies respectively shifted in energy by $\pm B_0$. The spectrum of $\mathcal{H}_{\rm eff}^2$ thus follows from the spectrum of a particle in a magnetic field [5] which, in Landau gauge, consists of a series of discretely spaced Landau levels $e_n(k_2)$, where the eigenvalues $e_n(k_2)$ are independent of $k_2$ ($k_2$ being the momentum associated with translation symmetry along $Y_2$) and are thus infinitely degenerate. At a fixed value of $k_2$, the spectrum of $\mathcal{H}_{\rm eff}^2$ therefore consists of a collection of discretely spaced eigenvalues ${\rm v}_{\rm D}^2\ [2B_0(n + 1/2) \pm B_0]$ with $n = 0, 1, 2, \ldots$, and corresponding eigenstates with centering $\propto k_2$. This is equivalent to a spectrum (at a fixed $k_2$) consisting of eigenvalues $2{\rm v}_{\rm D}^2 B_0 n$, with $n = 0, 1, 2, \ldots$, where each eigenvalue other than the $n = 0$ eigenvalue is two-fold degenerate ($n = 0$ having no degeneracy). Upon taking the square root, the two-fold degenerate pairs split into distinct positive and negative eigenvalues, yielding for the spectrum of $\mathcal{H}_{\rm eff}$:

$$(E_1)_n = \pm\sqrt{2{\rm v}_{\rm D}^2 B_0 n} \text{ with } n \in \{0, 1, 2, \ldots\}. \tag{5.11}$$

For the photonic crystal case, we can map the eigenvalue corrections $(E_1)_n$ to mode frequencies $\omega_n$ using: $(\omega/c)^2 = E = E_{\rm D} + \kappa E_1 + \mathcal{O}(\kappa^2)$, and $E_{\rm D} = (\omega_{\rm D}/c)^2$. This yields

$$\omega_n = \omega_{\rm D} \pm \frac{c^2 {\rm v}_{\rm D}}{\sqrt{2}\omega_{\rm D}} \sqrt{n\,|\mathbf{B}_{\rm eff}(\kappa)|} + O(\kappa^2) \text{ with } n = 0, 1, 2, \ldots, \tag{5.12}$$

where $|\mathbf{B}_{\rm eff}(\kappa)| = B_0\, \kappa^2$; see also the main text.

### 5.2. **Flattening weakly dispersive Landau levels using a modified strain.**

The effective theory predicts perfectly flat Landau levels. However, the Landau levels in Fig. 2 of the main text have dispersion arising from terms that are higher order in $\kappa$. To mitigate this dispersion, we note that the effective theory indicates that adding a quadratic strain-induced potential will tend to give the Landau levels curvature. Heuristically, this can be seen by recalling, for the standard Landau gauge Hamiltonian for a particle in a uniform magnetic field, that the eigenstate at a given $k_2$ in a given Landau level is localized in the $x_1$ direction and centered on $\tilde{x}$, where $\tilde{x} \propto k_2$ . Based on the $k_2-$dependent centering of these eigenstates, one would expect that introducing an $x_1$-dependent onsite effective electric

potential would add a $k_2$-dependent shift to the band frequencies since an eigenstate at $k_2$ should only be sensitive to the value of the potential over the finite region within which the state is localized.

Can the introduction of such an additional strain can be used to counter the curvature arising from higher order terms? Answering this question requires going beyond our effective equations. We therefore use full numerical simulations to compute the effect of adding the heuristically motivated strain and find that the unwanted dispersion can indeed be mitigated. As discussed in the main text, we modify the displacement to be $\mathbf{u}(\kappa\mathbf{x}) = a[\beta(\kappa x_1)^3, (\kappa x_1)^2]$, yielding a pseudomagnetic field $\mathbf{B}(\mathbf{x}) = -(4a\kappa^2 b_\star/\mathrm{v_D})\hat{\mathbf{z}}$ as well as a quadratic potential $W_{\mathrm{eff}}(\mathbf{x}) = 3a\beta\kappa(\omega_D/c)^2(\kappa x_1)^2$. Taking $\kappa = 0.0548a^{-1}$ and $\beta = 0.0380$ yields the band structures shown in Fig. 4 of the main text, where we see a clear flattening of the Landau levels.

5.3. **Proof of Theorem 5.1 by simplification of** (4.15)**.** We next evaluate the terms in (4.15), one at a time, using Proposition 4.2 and Proposition 4.3. Using Propositions 4.2 and 4.3, we simplify Term 1 and Term 2 of (4.15).

Term 1 of (4.15), $l = 1$:

$$\begin{aligned} -i\sum_{j=1}^{2}\langle\Phi_1,\mathcal{A}\Phi_j\rangle\cdot\nabla_{\mathbf{Y}}\alpha_j &= -i\,\langle\Phi_1,\mathcal{A}\Phi_2\rangle\ \cdot\ \nabla_{\mathbf{Y}}\alpha_2 && (\text{ Prop. 4.2, (1) })\\ &= \mathrm{v_D}\ (-i\partial_{Y_1}+\partial_{Y_2})\ \alpha_2 && (\text{ Prop. 4.2, (2) }) \end{aligned} \tag{5.13}$$

Term 1 of (4.15), $l = 2$:

$$\begin{aligned} -i\sum_{j=1}^{2}\langle\Phi_2,\mathcal{A}\Phi_j\rangle\cdot\nabla_{\mathbf{Y}}\alpha_j &= -i\,\langle\Phi_2,\mathcal{A}\Phi_1\rangle\ \cdot\ \nabla_{\mathbf{Y}}\alpha_1 && (\text{ Prop. 4.2, (1) })\\ &= \mathrm{v_D}\ (-i\partial_{Y_1}-\partial_{Y_2})\ \alpha_1 && (\text{ Prop. 4.2, (2) }) \end{aligned} \tag{5.14}$$

Term 2 of (4.15), $l = 1$:

$$\begin{aligned} -2\ \langle\Phi_1,\nabla_{\mathbf{y}}\cdot\xi\ U(\mathbf{Y})\ \nabla_{\mathbf{y}}\Phi_j\rangle\ &=\ 2\sum_{m,n}U_{mn}(\mathbf{Y})\ \langle\ \partial_{y_m}\Phi_1\ ,\ \xi\ \partial_{y_n}\Phi_j\ \rangle\\ &=\ 2\sum_{m,n}U_{mn}(\mathbf{Y})\ A^{1j}_{mn} \end{aligned} \tag{5.15}$$

where we have used (4.16) and the definition of $A^{lj}_{mn}$ in (4.17). Therefore,

$$2\sum_{j}\ \langle\Phi_1,\nabla_{\mathbf{y}}\cdot\xi\ U(\mathbf{Y})\ \nabla_{\mathbf{y}}\Phi_j\rangle\ \alpha_j(\mathbf{Y})\ =\ -2\sum_{m,n}U_{mn}(\mathbf{Y})\sum_{j}\ A^{1j}_{mn}\ \alpha_j(\mathbf{Y}) \tag{5.16}$$

Consider now the sum over $j$: $\sum_j\ A^{1j}_{mn}\ \alpha_j(\mathbf{Y}) = A^{11}_{mn}\alpha_1(\mathbf{Y}) + A^{12}_{mn}\alpha_2(\mathbf{Y})$. By Proposition 4.3:

$$\begin{aligned} A^{11}_{mn}\ &=\ \left(\ a_\star\ \sigma_0\ +\tilde{a}^{11}\ i\sigma_2\ \right)_{mn}\quad\text{and}\\ A^{12}_{mn}\ &=\ b_\star\ (\ \sigma_3\ -\ i\ \sigma_1\ )_{mn}\,. \end{aligned}$$

Therefore,

$$\sum_j A^{1j}_{mn}\ \alpha_j(\mathbf{Y})\ =\ \left(\ a_\star\ \sigma_0\ +\tilde{a}^{11}\ i\sigma_2\ \right)_{mn}\ \alpha_1(\mathbf{Y})\ +\ b_\star\ \left(\ \sigma_3\ -\ i\ \sigma_1\ \right)_{mn}\ \alpha_2(\mathbf{Y})$$

and finally we have

Term 2 of (4.15), $l=1$:

$$\begin{aligned} 2\sum_j\ \langle\Phi_1,\nabla_{\mathbf{y}}\cdot\xi\ U(\mathbf{Y})\ \nabla_{\mathbf{y}}\Phi_j\rangle\ \alpha_j(\mathbf{Y})\ &=\ -2\sum_{m,n} U_{mn}(\mathbf{Y})\ \sum_j\ A^{1j}_{mn}\ \alpha_j(\mathbf{Y}) \\ &=\ -2\sum_{m,n} U_{mn}\ \left(\ a_\star\ \sigma_0\ +\tilde{a}^{11}\ i\sigma_2\ \right)_{mn}\ \alpha_1\ -\ 2\ b_\star \sum_{m,n} U_{mn}\ \left(\ \sigma_3\ -\ i\ \sigma_1\ \right)_{mn}\ \alpha_2 \\ &=\ -2\ a_\star\ \mathrm{tr}(U)\ \alpha_1\ -\ 2\ b_\star\ \left(\ \mathrm{tr}(\sigma_3 U)\ -\ i\ \mathrm{tr}(\sigma_1 U)\ \right)\ \alpha_2, \end{aligned} \tag{5.17}$$

where we have used: $\sigma_2^\top=-\sigma_2$, $U^\top=U$ and finally $\mathrm{tr}(V^\top U)=\sum_{m,n}V_{mn}U_{mn}$. Similarly, we have for

Term 2 of (4.15), $l=2$:

$$\begin{aligned} 2\sum_j\ \langle\Phi_2,\nabla_{\mathbf{y}}\cdot\xi\ U(\mathbf{Y})\ \nabla_{\mathbf{y}}\Phi_j\rangle\ \alpha_j(\mathbf{Y})\ &=\ -2\sum_{m,n} U_{mn}(\mathbf{Y})\ \sum_j\ A^{2j}_{mn}\ \alpha_j(\mathbf{Y}) \\ &=\ -2\ a_\star\ \mathrm{tr}(U)\ \alpha_2\ -\ 2\ b_\star\ \left(\ \mathrm{tr}(\sigma_3 U)+\ i\ \mathrm{tr}(\sigma_1 U)\ \right)\alpha_1. \end{aligned} \tag{5.18}$$

We now complete the proof of Theorem 5.1. Substitution of (5.13) and (5.17) into (4.15) for $l=1$, and (5.14) and (5.18) into (4.15) for $l=2$ yields the system:

$$\begin{aligned} \left[\ \mathrm{v_D}\ (-i\partial_{Y_1}+\partial_{Y_2})\ -\ 2\ b_\star\ \left(\ \mathrm{tr}(\sigma_3 U)\ -\ i\ \mathrm{tr}(\sigma_1 U)\ \right)\ \right]\ \alpha_2-\ 2\ a_\star\ \mathrm{tr}(U)\ \alpha_1\ &=\ E_1\ \alpha_1 \\ \left[\ \overline{\mathrm{v_D}}\ (-i\partial_{Y_1}-\partial_{Y_2})\ -\ 2\ \overline{b_\star}\ \left(\ \mathrm{tr}(\sigma_3 U)\ +\ i\ \mathrm{tr}(\sigma_1 U)\ \right)\ \right]\ \alpha_1-\ 2\ a_\star\ \mathrm{tr}(U)\ \alpha_2\ &=\ E_1\ \alpha_2, \end{aligned} \tag{5.19}$$

where we recall from Proposition 2.5 that $\mathrm{v_D}=\overline{\mathrm{v_D}}$ and $b_\star=\overline{b_\star}$. Using Pauli matrices, $\sigma_i$, the system (5.19) can be expressed as (5.1).

## Appendix A. Matrix elements via symmetry; proof of Proposition 4.3

Let $\mathbf{x}\mapsto R\mathbf{x}$ denote a rotation on $\mathbb{R}^2$ by $2\pi/3$

$$R\ =\ \begin{pmatrix} -\frac{1}{2} & \frac{\sqrt{3}}{2} \\ -\frac{\sqrt{3}}{2} & -\frac{1}{2} \end{pmatrix}$$

and recall the rotation operator: $\mathcal{R}[f](\mathbf{x})\ =\ f(R^*\mathbf{x})$. Recall from Proposition 2.3 that

$$\mathcal{R}[\Phi_j](\mathbf{x})\ =\ \tau^j\Phi_j(\mathbf{x}),\ j=1,2,\ \text{where } \tau=e^{2\pi i/3}.$$

**Proposition A.1.** *Let $A^{ij}$ $(i,j=1,2)$ denote the matrices given in* (4.17)*. Then,*

*(1)*

$$A^{ij}\ =\ \tau^{j-i}\ R^\top A^{ij}R$$

*(2) $i=j$:* $\quad A^{jj}\ =\ R^\top A^{jj}R$

*(3) $i\neq j$:* $\quad A^{12}\ =\ \tau\ R^\top A^{12}R,\ $ *and* $A^{21}\ =\ \overline{\tau}\ R^\top A^{21}R$

*Proof of Proposition A.1:* Fix $\kappa = (\kappa_1, \kappa_2) \in \mathbb{R}^2$. Then, with summation over repeated indices implied,

$$\begin{aligned}
\kappa^\top\ A^{ij}\ \kappa\ &=\ \left\langle \partial_{y_\alpha}\Phi_i, \xi\ \partial_{y_\beta}\Phi_j \right\rangle\ \kappa_\alpha\kappa_\beta \\
&=\ \left\langle \mathcal{R}\ \partial_{y_\alpha}\Phi_i, \xi\ \mathcal{R}\ \partial_{y_\beta}\Phi_j \right\rangle\ \kappa_\alpha\kappa_\beta \\
&= \left\langle\ R_{n\alpha}\partial_{y_n}\ \mathcal{R}[\Phi_i], \xi\ R_{q\beta}\partial_{y_q}\ \mathcal{R}[\Phi_j] \right\rangle\ \kappa_\alpha\kappa_\beta \\
&=\ \left\langle\ R_{n\alpha}\partial_{y_n}\ \tau^i\Phi_i, \xi\ R_{q\beta}\partial_{y_q}\ \tau^j\Phi_j \right\rangle\ \kappa_\alpha\kappa_\beta \\
&=\ \tau^{j-i}\ \left\langle\ R_{n\alpha}\partial_{y_n}\ \Phi_i, \xi\ R_{q\beta}\partial_{y_q}\ \Phi_j \right\rangle\ \kappa_\alpha\kappa_\beta \\
&=\ \tau^{j-i}\ \left\langle\ \partial_{y_n}\ \Phi_i, \xi\ \partial_{y_q}\ \Phi_j \right\rangle\ R_{n\alpha}\kappa_\alpha\ R_{q\beta}\kappa_\beta \\
&=\ \tau^{j-i}\ \left\langle\ \partial_{y_n}\ \Phi_i, \xi\ \partial_{y_q}\ \Phi_j \right\rangle\ (R\kappa)_n\ (R\kappa)_q \\
&=\ \tau^{j-i}\ \ (R\kappa)^\top\ A^{ij}(R\kappa) \\
&=\ \tau^{j-i}\ \ \kappa^\top\ \left(\ R^\top A^{ij} R\ \right) \kappa
\end{aligned}$$

Since $\kappa$ is arbitrary, we conclude:

$$A^{ij}\ =\ \tau^{j-i}\ R^\top A^{ij} R, \qquad i,j = 1,2.$$

We have three cases:

$$\begin{cases} i = j: & A^{jj}\ =\ R^\top A^{jj} R, \quad j = 1,2 \\ (i,j) = (1,2): & A^{12}\ =\ \tau\ R^\top A^{12} R \\ (i,j) = (2,1): & A^{21}\ =\ \overline{\tau}\ R^\top A^{21} R \end{cases} \tag{A.1}$$

This completes the proof of Proposition A.1.

We now deduce Proposition 4.3 using Proposition A.1.
*Proof of Proposition 4.3:* The $2\pi/3$ rotation matrix is given by

$$R\ =\ \begin{pmatrix} -\frac{1}{2} & \frac{\sqrt{3}}{2} \\ -\frac{\sqrt{3}}{2} & -\frac{1}{2} \end{pmatrix} \tag{A.2}$$

*Case 1, i=j:* By (A.1) we have

$$\begin{pmatrix} -\frac{1}{2} & \frac{\sqrt{3}}{2} \\ -\frac{\sqrt{3}}{2} & -\frac{1}{2} \end{pmatrix} \begin{pmatrix} a & b \\ c & d \end{pmatrix}\ =\ \begin{pmatrix} a & b \\ c & d \end{pmatrix}\ \begin{pmatrix} -\frac{1}{2} & \frac{\sqrt{3}}{2} \\ -\frac{\sqrt{3}}{2} & -\frac{1}{2} \end{pmatrix},$$

where $a, b, c$ and $d$ are to be determined. Equating entries, yields that $c = -b$ and $a = d$. Hence,

$$A^{jj}\ =\ a^{jj}\ I_{2\times 2}\ +\ \tilde{a}^{jj}\ \begin{pmatrix} 0 & 1 \\ -1 & 0 \end{pmatrix}, \quad j = 1,2.$$

We claim further that $a^{11} = a^{22}$. Indeed, we have:

$$\begin{aligned} a^{11} &= \int_\Omega \overline{\frac{\partial \Phi_1(\mathbf{x})}{\partial x_1}}\ \xi(\mathbf{x})\ \frac{\partial \Phi_1(\mathbf{x})}{\partial x_1}\ d\mathbf{x} \\ &= \int_\Omega \overline{\frac{\partial \Phi_1(-\mathbf{y})}{\partial y_1}}\ \xi(-\mathbf{y})\ \frac{\partial \Phi_1(-\mathbf{y})}{\partial y_1}\ d\mathbf{y} \\ &= \int_\Omega \overline{\frac{\partial \Phi_1(-\mathbf{y})}{\partial y_1}}\ \xi(-\mathbf{y})\ \overline{\frac{\partial \overline{\Phi_1(-\mathbf{y})}}{\partial y_1}}\ d\mathbf{y} \\ &= \int_\Omega \frac{\partial \Phi_2(\mathbf{y})}{\partial y_1}\ \xi(\mathbf{y})\ \overline{\frac{\partial \Phi_2(\mathbf{y})}{\partial y_1}}\ d\mathbf{y}\ =\ a^{22}. \end{aligned}$$

We therefore set $a_\star \equiv a^{11} = a^{22}$. Finally, taking the inner product of the equation $(-\nabla\cdot\xi\nabla + V)\,\Phi_j = E\ \rho\ \Phi_j$ with $\Phi_j$ and using that $\langle \Phi_i, \Phi_j\rangle_\rho = \delta_{ij}$ gives:

$$\int_\Omega \xi(\mathbf{y})\ |\nabla\Phi_j(\mathbf{y})|^2\ d\mathbf{y}\ +\ \int_\Omega V(\mathbf{y})\ |\Phi_j(\mathbf{y})|^2\ d\mathbf{y} =\ E_D\ ,\ j=1,2.$$

Hence,

$$a_\star\ =\ \frac{1}{2}\ E_D\ -\ \frac{1}{2}\ \int_\Omega V(\mathbf{y})\ |\Phi_j(\mathbf{y})|^2\ d\mathbf{y}\ ,\ j=1,2. \tag{A.3}$$

This proves (4.19), (4.20) and (4.21), and in conclusion we have:

$$A^{jj}\ =\ a_\star\ I_{2\times 2}\ +\ \tilde{a}^{jj}\ \begin{pmatrix} 0 & 1 \\ -1 & 0 \end{pmatrix},\quad j=1,2\ ,$$

where $\tilde{a}^{22} = -\tilde{a}^{11}$. This proves part (1) of Proposition 4.3.

*Case 2, (i,j)=(1,2):* By (A.1) we have

$$\begin{pmatrix} -\frac{1}{2} & \frac{\sqrt{3}}{2} \\ -\frac{\sqrt{3}}{2} & -\frac{1}{2} \end{pmatrix} \begin{pmatrix} a & b \\ c & d \end{pmatrix}\ =\ \tau\ \begin{pmatrix} a & b \\ c & d \end{pmatrix}\ \begin{pmatrix} -\frac{1}{2} & \frac{\sqrt{3}}{2} \\ -\frac{\sqrt{3}}{2} & -\frac{1}{2} \end{pmatrix}.$$

Equating entries, we obtain a system of four homogeneous linear equations, $M\mathbf{z} = \mathbf{0}$, for the unknowns $\mathbf{z} = (a,b,c,d)^\top$. The matrix $M$ has rank three and its null space is spanned by the vector $(1,-i,-i,-1)^\top$. Thus,

$$A^{12}\ =\ b_\star\ \begin{pmatrix} 1 & -i \\ -i & -1 \end{pmatrix}, \text{where}\ \ b_\star\ =\ \langle \partial_{y_1}\Phi_1, \xi\ \partial_{y_1}\Phi_2\rangle\ .$$

Furthermore, since $A^{lj}_{\alpha\beta}\ =\ \overline{A^{jl}_{\beta\alpha}}$, we find:

$$A^{21}\ =\ \overline{b_\star}\ \begin{pmatrix} 1 & i \\ i & -1 \end{pmatrix}\ .$$

This proves part (2) of Proposition 4.3.

## Appendix B. $v_D \geq 0$ and $b_\star \geq 0$; Proof of Proposition 2.5

We begin by recalling the expressions for $v_D$ and $b_\star$ in (2.13) and (2.14):

$$v_D = \langle \Phi_1, \mathcal{A}_1 \Phi_2 \rangle, \qquad b_\star \ = \ \langle \partial_{x_1}\Phi_1,\ \xi\ \partial_{x_1}\Phi_2 \rangle\ .$$

We will consider two coordinate systems (with coordinates denoted by $\mathbf{x}$ and $\mathbf{x}'$) that differ by a rotation. We define $v_D$ and $b_\star$ as the quantities in the $\mathbf{x}$ coordinate system and $v_D'$ and $b_\star'$ as the quantities in the $\mathbf{x}'$ coordinate system. We will assume that $v_D'$ and $b_\star'$ are complex and then demonstrate that, by rotating the unprimed coordinate system relative to the primed coordinate system (as well as making an appropriate phase choice for the eigenstates), $v_D$ and $b_\star$ can be made to be real.

Introduce a rotation of coordinates from $\mathbf{x} = (x_1, x_2)$ to $\mathbf{x}' = (x_1', x_2')$ related by:

$$\mathbf{x}' \ = \ \begin{pmatrix} x_1' \\ x_2' \end{pmatrix} \ = \ \begin{pmatrix} \cos\theta & -\sin\theta \\ \sin\theta & \cos\theta \end{pmatrix} \begin{pmatrix} x_1 \\ x_2 \end{pmatrix} \ = \ R_\theta\ \mathbf{x}.$$

We therefore have

$$\frac{\partial}{\partial x_1} \ = \ \frac{\partial x_1'}{\partial x_1}\frac{\partial}{\partial x_1'} \ + \ \frac{\partial x_2'}{\partial x_1}\frac{\partial}{\partial x_2'} = \ \cos\theta\ \frac{\partial}{\partial x_1'} \ + \ \sin\theta\ \frac{\partial}{\partial x_2'} \ = \ \zeta\cdot\nabla_{\mathbf{x}'}, \quad \zeta = (\cos\theta, \sin\theta).$$

Now given any function $f(\mathbf{x})$, we define

$$f'(\mathbf{x}') = \mathcal{R}_\theta[f](\mathbf{x}') \ = \ f\left(R_\theta^* \mathbf{x}'\right),$$

and introduce the rotated Bloch eigenfunctions:

$$\Phi_j'(\mathbf{x}') \ = \ \mathcal{R}_\theta[\Phi_j](\mathbf{x}')\ ,\ j = 1, 2.$$

These satisfy the equations for the structure defined by $\xi' = \mathcal{R}_\theta[\xi]$, $\rho' = \mathcal{R}_\theta[\rho]$, and $V' = \mathcal{R}_\theta[V]$:

$$\left[-\nabla_{\mathbf{x}'}\cdot\xi'\ \nabla_{\mathbf{x}'} + V'\right]\Phi_j' \ = \ E_D\ \rho'\ \Phi_j'.$$

Using the notation,

$$\mathcal{A}_m' \ = \ \frac{1}{i}\xi'\partial_{x_m'} \ + \ \frac{1}{i}\partial_{x_m'}(\xi'\ \cdot)$$

and the identities (equation (2.11)): $\langle \Phi_1',\ \mathcal{A}_1'\Phi_2'\rangle = v_D'$, $\quad \langle \Phi_1',\ \mathcal{A}_2'\Phi_2'\rangle = i v_D'$, we have:

$$v_D \ \equiv \ \langle \Phi_1,\ \mathcal{A}_1\Phi_2\rangle \ = \ \langle \Phi_1',\ \zeta\cdot\mathcal{A}'\Phi_2'\rangle \ = \ \cos\theta\ \langle \Phi_1',\ \mathcal{A}_1'\Phi_2'\rangle \ + \ \sin\theta\ \langle \Phi_1',\ \mathcal{A}_2'\Phi_2'\rangle \ = \ v_D'\ e^{i\theta}. \tag{B.1}$$

We now turn to considering $b_\star$ in a rotated coordinate system. Recalling the notation:

$$A_{\alpha\beta}^{lj} \ = \ \left\langle \partial_{y_\alpha}\Phi_l, \xi\ \partial_{y_\beta}\Phi_j \right\rangle, \quad j, l, \alpha, \beta = 1, 2\ ,$$

we have

$$\begin{aligned} b_\star \ &= \ \langle \partial_{x_1}\Phi_1,\ \xi\ \partial_{x_1}\Phi_2\rangle \ = \ \langle (\zeta\cdot\nabla_{\mathbf{x}'})\Phi_1',\ \xi'\ (\zeta\cdot\nabla_{\mathbf{x}'})\Phi_2'\rangle \\ &= \ \cos^2\theta \left\langle \partial_{x_1'}\Phi_1',\ \xi'\ \partial_{x_1'}\Phi_2'\right\rangle \ + \ \sin^2\theta \left\langle \partial_{x_2'}\Phi_1',\ \xi'\ \partial_{x_2'}\Phi_2'\right\rangle \\ &\quad + \ \sin\theta\ \cos\theta \left( \ \left\langle \partial_{x_2'}\Phi_1',\ \xi'\ \partial_{x_1'}\Phi_2'\right\rangle \ + \ \left\langle \partial_{x_1'}\Phi_1',\ \xi'\ \partial_{x_2'}\Phi_2'\right\rangle \ \right) \\ &= \cos^2\theta\ (A')_{11}^{12} \ + \ \sin^2\theta\ (A')_{22}^{12} \ + \ \sin\theta\ \cos\theta\left(\ (A')_{21}^{12} + (A')_{12}^{12}\ \right) \end{aligned}$$

The previous expression may be simplified using Proposition 4.3, yielding

$$b_\star \ = \ (\cos^2\theta - \sin^2\theta)\ b_\star' \ - 2i\sin\theta\cos\theta\ b_\star' \ = \ e^{-2i\theta}\ b_\star' \tag{B.2}$$

Explicitly, (B.1) and (B.2) state:

$$\begin{aligned} \langle \Phi_1,\ \mathcal{A}_1 \Phi_2 \rangle \ &= \ e^{i\theta}\ \langle \Phi_1',\ \mathcal{A}_1' \Phi_2' \rangle \\ \langle \partial_{x_1}\Phi_1,\ \xi\ \partial_{x_1}\Phi_2 \rangle \ &= \ e^{-2i\theta}\ \left\langle \partial_{x_1'}\Phi_1',\ \xi'\ \partial_{x_1'}\Phi_2' \right\rangle , \end{aligned} \tag{B.3}$$

where $\theta$ is to be chosen. Here, $\Phi_1'(\mathbf{x}) \in L^2_{\mathbf{K},\tau}$ and $\Phi_2'(\mathbf{x}) = \overline{\Phi_1'(-\mathbf{x})} \in L^2_{\mathbf{K},\overline{\tau}}$ are any choice of Bloch states in the primed coordinate system.

We next exploit the phase degree of freedom in the choice of these states. In particular,

replace $\Phi_1'$ by $e^{i\phi}\Phi_1' \in L^2_{\mathbf{K},\tau}$ and hence $\Phi_2'$ by $e^{-i\phi}\Phi_2' \in L^2_{\mathbf{K},\overline{\tau}}$,

where now both $\theta$ and $\phi$ are to be determined. Therefore, (B.3) becomes

$$\begin{aligned} \mathrm{v_D} \ &\equiv \ \langle \Phi_1,\ \mathcal{A}_1 \Phi_2 \rangle \ = \ e^{i(\theta - 2\phi)}\ \langle \Phi_1',\ \mathcal{A}_1' \Phi_2' \rangle \ = \ e^{i(\theta-2\phi)}\ \mathrm{v_D'} \\ b_\star \ &\equiv \langle \partial_{x_1}\Phi_1,\ \xi\ \partial_{x_1}\Phi_2 \rangle \ = \ e^{-2i(\theta+\phi)}\ \left\langle \partial_{x_1'}\Phi_1',\ \xi'\ \partial_{x_1'}\Phi_2' \right\rangle \ = \ e^{-2i(\theta+\phi)}\ b_\star' \ . \end{aligned} \tag{B.4}$$

Hence, if we choose

$$\theta = -\frac{1}{3}\arg \mathrm{v_D'} + \frac{1}{3}\arg b_\star', \quad \phi = \frac{1}{3}\arg \mathrm{v_D'} + \frac{1}{6}\arg b_\star',$$

then we obtain $\mathrm{v_D} \geq 0$ and $b_\star \geq 0$. This completes the proof of Proposition 2.5.

We now confirm that the effective Hamiltonian transforms as expected under a rotation of coordinates. Let $\mathcal{H}_{\text{eff}}$ and $\mathcal{H}_{\text{eff}}'$ be the effective Hamiltonians written in the $\mathbf{x}$ and $\mathbf{x}'$ coordinate systems, respectively. We choose the $\mathbf{x}$ coordinates so that $\mathrm{v_D}$ and $b_\star$ are real (as shown above, this is always possible). As before, we take the two coordinate systems to be related by $\mathbf{x}' = R_\theta \mathbf{x}$ with

$$R_\theta = \begin{pmatrix} \cos\theta & -\sin\theta \\ \sin\theta & \cos\theta \end{pmatrix} \tag{B.5}$$

In the primed coordinate system, $\mathrm{v_D'}$ and $b_\star'$ are in general complex. Let $U$ and $U'$ be the strain matrices computed in the $\mathbf{x}$ and $\mathbf{x}'$ coordinate systems, respectively, and denote $\mathbf{p} = -i\nabla_{\mathbf{x}}$ and $\mathbf{p}' = -i\nabla_{\mathbf{x}'}$. From Eq. 5.19 (combined with the convention for the eigenvalue problem in Eq. 5.5), we have

$$\begin{aligned} \mathcal{H}_{\text{eff}}' = &\begin{pmatrix} 0 & \overline{\mathrm{v_D'}}\,(p_1' - ip_2') \\ \mathrm{v_D'}\,(p_1' + ip_2') & 0 \end{pmatrix} + \begin{pmatrix} 0 & -2\overline{b_\star'}\big(\mathrm{tr}(\sigma_3 U') + i\,\mathrm{tr}(\sigma_1 U')\big) \\ -2b_\star'\big(\mathrm{tr}(\sigma_3 U') - i\,\mathrm{tr}(\sigma_1 U')\big) & 0 \end{pmatrix} \\ &- 2a_\star'\mathrm{tr}(U'\sigma_0)\begin{pmatrix} 1 & 0 \\ 0 & 1 \end{pmatrix} . \end{aligned} \tag{B.6}$$

The effective Hamiltonian in the unprimed coordinates is given by Eq. 5.5

$$\mathcal{H}_{\text{eff}} \ = \ \mathrm{v_D}\,(\mathbf{p} - \mathbf{A}_{\text{eff}})\cdot\sigma \ + \ W_{\text{eff}}\ \sigma_0 \tag{B.7}$$

with

$$\begin{aligned} W_{\text{eff}} &= -2a_\star\ \mathrm{tr}\,(U\sigma_0) \\ \mathbf{A}_{\text{eff}} \ &= \ \frac{2b_\star}{\mathrm{v_D}}\ \begin{pmatrix} +\mathrm{tr}\,(U\sigma_3) \\ -\mathrm{tr}\,(U\sigma_1) \end{pmatrix} . \end{aligned} \tag{B.8}$$

As discussed above, we have

$$\mathrm{v_D'} = \mathrm{v_D} e^{-i\theta} \qquad b_\star' = b_\star e^{2i\theta} \tag{B.9}$$

We now simplify each of the three terms in Eq. B.6. Using Eq. B.9 gives for the first term:

$$\begin{pmatrix} 0 & \overline{\mathrm{v}'_{\mathrm{D}}}\,(p'_1 - ip'_2) \\ \mathrm{v}'_{\mathrm{D}}\,(p'_1 + ip'_2) & 0 \end{pmatrix} = \mathrm{v}_{\mathrm{D}}\Big(p'_1(\cos\theta\,\sigma_1 - \sin\theta\,\sigma_2) + p'_2(\sin\theta\,\sigma_1 + \cos\theta\,\sigma_2)\Big)$$
$$= \mathrm{v}_{\mathrm{D}}\,\mathbf{p}'\cdot\sigma' \tag{B.10}$$

where in the last line we have defined rotated Pauli matrices $\sigma'_j = \mathcal{V}\sigma_j\mathcal{V}^*$ with $\mathcal{V} = e^{i\theta(\sigma_3/2)}$. Equivalently, the rotated Pauli matrices are given by:

$$\begin{pmatrix}\sigma'_1\\ \sigma'_2\end{pmatrix} = \begin{pmatrix}\cos\theta & -\sin\theta\\ \sin\theta & \cos\theta\end{pmatrix}\begin{pmatrix}\sigma_1\\ \sigma_2\end{pmatrix}. \tag{B.11}$$

Using Eq. B.9, we have for the second term of Eq. B.6

$$\begin{pmatrix} 0 & -2\overline{b'_\star}\big(\mathrm{tr}(\sigma_3U') + i\,\mathrm{tr}(\sigma_1U')\big) \\ -2b'_\star\big(\mathrm{tr}(\sigma_3U') - i\,\mathrm{tr}(\sigma_1U')\big) & 0 \end{pmatrix}$$
$$= -2b_\star\Big([\,\mathrm{tr}(\sigma_3U')\cos2\theta + \mathrm{tr}(\sigma_1U')\sin2\theta\,]\sigma_1 + [\,\mathrm{tr}(\sigma_3U')\sin2\theta - \mathrm{tr}(\sigma_1U')\cos2\theta\,]\sigma_2\Big)$$
$$= -2b_\star\Big([\,\mathrm{tr}(\sigma_3U')\cos3\theta + \mathrm{tr}(\sigma_1U')\sin3\theta\,]\sigma'_1 + [\,\mathrm{tr}(\sigma_3U')\sin3\theta - \mathrm{tr}(\sigma_1U')\cos3\theta\,]\sigma'_2\Big)$$
$$= -\mathrm{v}_{\mathrm{D}}\,\mathbf{A}'_{\mathrm{eff}}\cdot\sigma' \tag{B.12}$$

where we have defined

$$\mathbf{A}'_{\mathrm{eff}} = \frac{2b_\star}{\mathrm{v}_{\mathrm{D}}}\begin{pmatrix}\cos3\theta & -\sin3\theta\\ \sin3\theta & \cos3\theta\end{pmatrix}\begin{pmatrix}+\mathrm{tr}(\sigma_3U')\\ -\mathrm{tr}(\sigma_1U')\end{pmatrix}. \tag{B.13}$$

To relate $\mathbf{A}'_{\mathrm{eff}}$ to $\mathbf{A}_{\mathrm{eff}}$, we note that $U' = R_\theta U R_\theta^T$. Hence, Eq. B.13 becomes

$$\mathbf{A}'_{\mathrm{eff}} = \frac{2b_\star}{\mathrm{v}_{\mathrm{D}}}\begin{pmatrix}\cos3\theta & -\sin3\theta\\ \sin3\theta & \cos3\theta\end{pmatrix}\begin{pmatrix}+\mathrm{tr}(R_\theta^T\sigma_3R_\theta U)\\ -\mathrm{tr}(R_\theta^T\sigma_1R_\theta U)\end{pmatrix}$$
$$= \frac{2b_\star}{\mathrm{v}_{\mathrm{D}}}\begin{pmatrix}\cos3\theta & -\sin3\theta\\ \sin3\theta & \cos3\theta\end{pmatrix}\begin{pmatrix}\cos2\theta & \sin2\theta\\ -\sin2\theta & \cos2\theta\end{pmatrix}\begin{pmatrix}+\mathrm{tr}(\sigma_3U)\\ -\mathrm{tr}(\sigma_1U)\end{pmatrix}$$
$$= \frac{2b_\star}{\mathrm{v}_{\mathrm{D}}}\begin{pmatrix}\cos\theta & -\sin\theta\\ \sin\theta & \cos\theta\end{pmatrix}\begin{pmatrix}+\mathrm{tr}(\sigma_3U)\\ -\mathrm{tr}(\sigma_1U)\end{pmatrix}$$
$$= R_\theta\,\mathbf{A}_{\mathrm{eff}}. \tag{B.14}$$

Note also that $\mathbf{p}' = R_\theta\mathbf{p}$. Finally, from the expression for $a_\star$ in Theorem 5.1, it is clear that $a'_\star = a_\star$. Hence, for the third term in Eq. B.6, we have

$$W'_{\mathrm{eff}} \equiv -2a'_\star\mathrm{tr}(U'\sigma_0) = -2a_\star\mathrm{tr}(UR_\theta^T\sigma_0R_\theta)$$
$$= W_{\mathrm{eff}}. \tag{B.15}$$

Putting all of this together, we have

$$\mathcal{H}_{\mathrm{eff}} = \mathrm{v}_{\mathrm{D}}\,(\mathbf{p} - \mathbf{A}_{\mathrm{eff}})\cdot\sigma + W_{\mathrm{eff}}\,\sigma_0$$
$$\mathcal{H}'_{\mathrm{eff}} = \mathrm{v}_{\mathrm{D}}\,(\mathbf{p}' - \mathbf{A}'_{\mathrm{eff}})\cdot\sigma' + W'_{\mathrm{eff}}\,\sigma'_0 \tag{B.16}$$

where

$$\mathbf{A}'_{\mathrm{eff}} = R_\theta\mathbf{A}_{\mathrm{eff}} \qquad \mathbf{p}' = R_\theta\mathbf{p} \qquad W'_{\mathrm{eff}} = W_{\mathrm{eff}} \qquad \sigma'_j = \mathcal{V}\sigma_j\mathcal{V}^* \tag{B.17}$$

with $\mathcal{V} = e^{i\theta(\sigma_3/2)}$.

## References

[1] A. Drouot and M. I. Weinstein, *Edge states and the valley Hall effect* (https://arxiv.org/abs/1910.03509).

[2] C. L. Fefferman, J. P. Lee-Thorp, and M. I. Weinstein, *Edge states in honeycomb structures*, Annals of PDE **2** (2016), no. 12.

[3] C. L. Fefferman and M. I. Weinstein, *Honeycomb lattice potentials and Dirac points*, J. Amer. Math. Soc. **25** (2012), no. 4, 1169–1220.

[4] ———, *Wave packets in honeycomb lattice structures and two-dimensional Dirac equations*, Commun. Math. Phys. **326** (2014), 251–286.

[5] L. D. Landau and E. M. Lifshitz, *Quantum mechanics: Non-relativistic theory*, Pergamon Press, 1977.

[6] J. P. Lee-Thorp, M. I. Weinstein, and Y. Zhu, *Elliptic operators with honeycomb symmetry; Dirac points, edge states and applications to photonic graphene*, Arch. Rational Mech. Anal. **232** (2019), no. 1, 1–63.
